# Supplementary material for: SVAD: From Single Image to 3D Avatar via Synthetic Data Generation with Video Diffusion and Data Augmentation
Source: arXiv:2505.05475 source file (2025-05-08)
Supplement: Supplementary file 1 [file app_text2avatar.pdf]

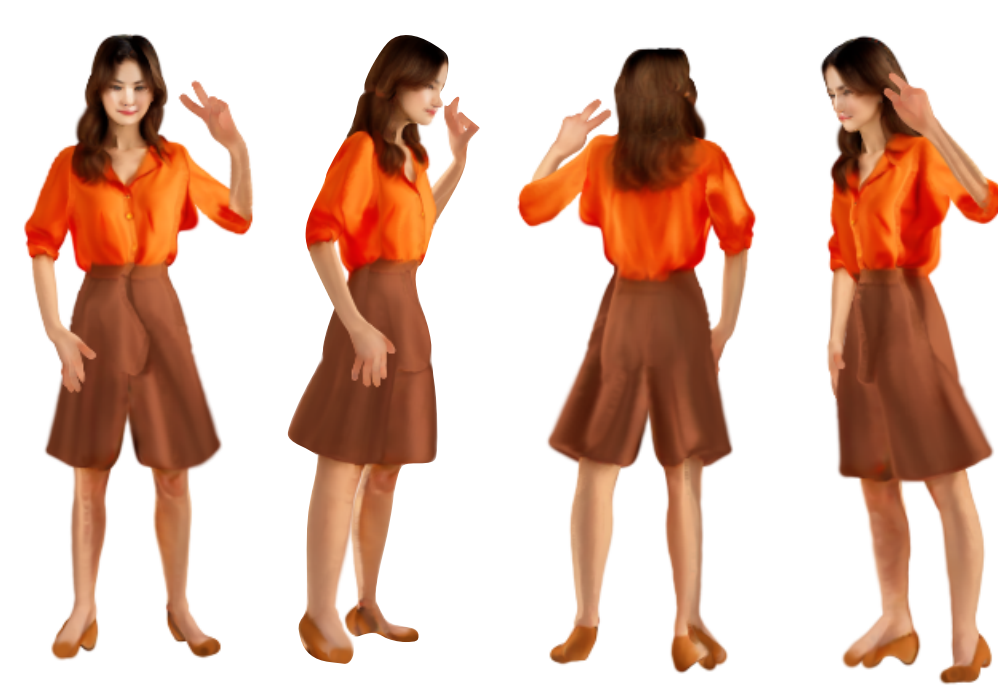

*“A woman with orange blouse and brown skirt”*

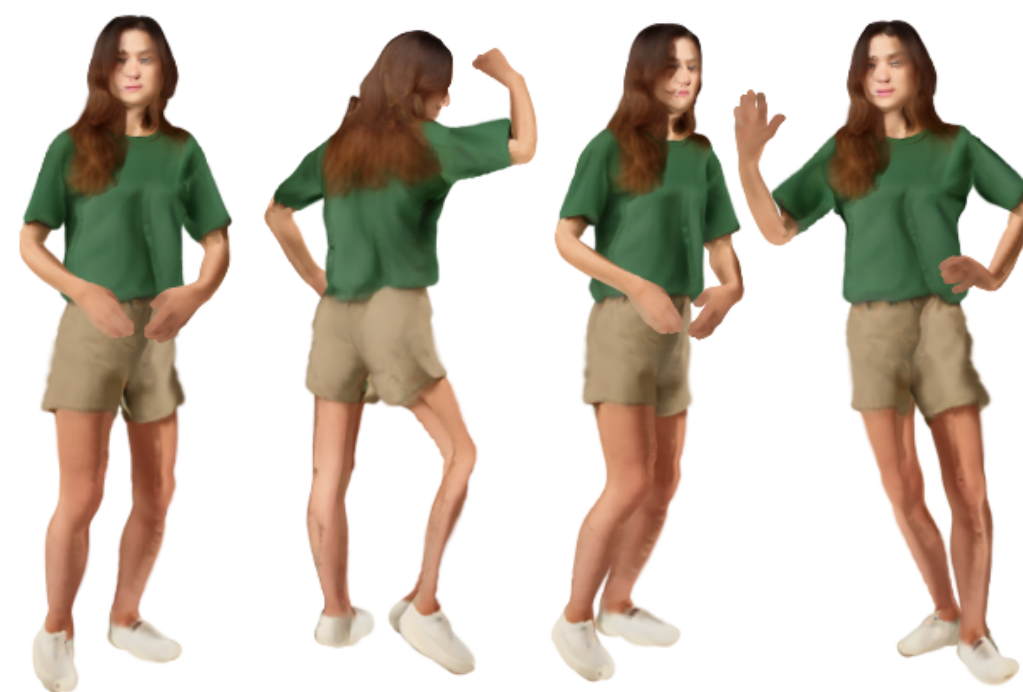

*“A woman with green t-shirt and khaki shorts”*

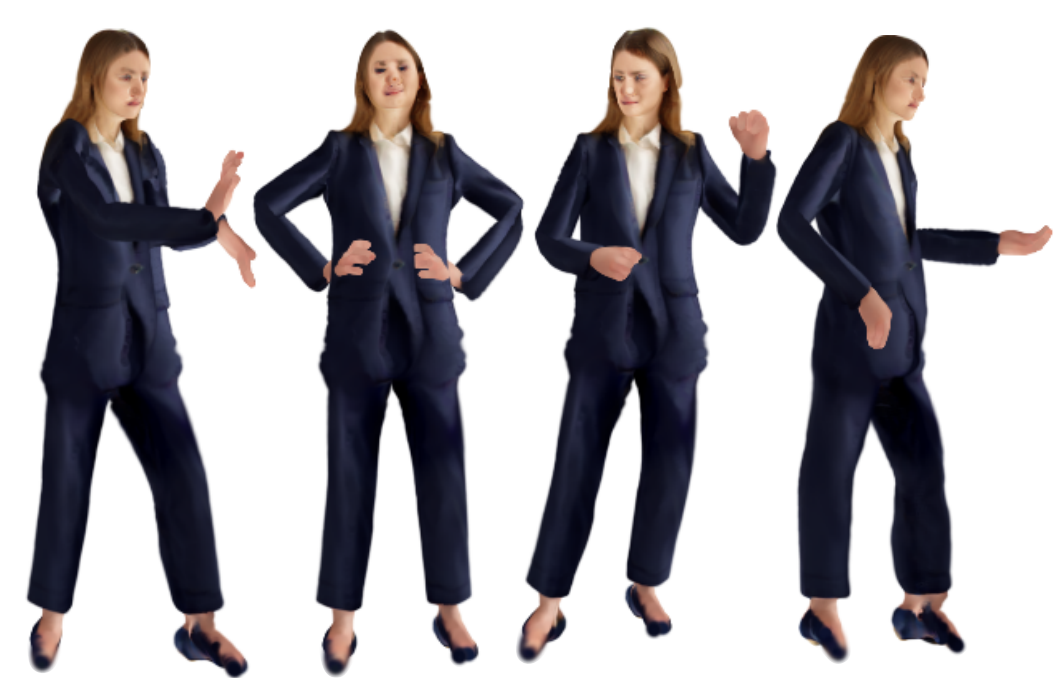

*“A woman with navy blue blazer and matching pants”*

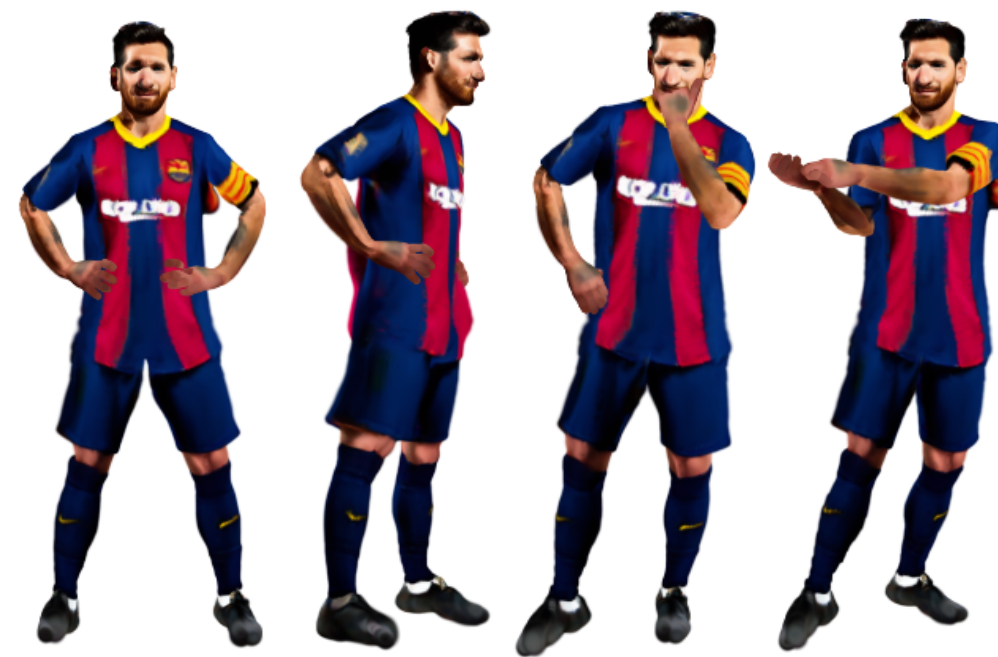

*“Lionel Messi in FC Barcelona uniform ”*

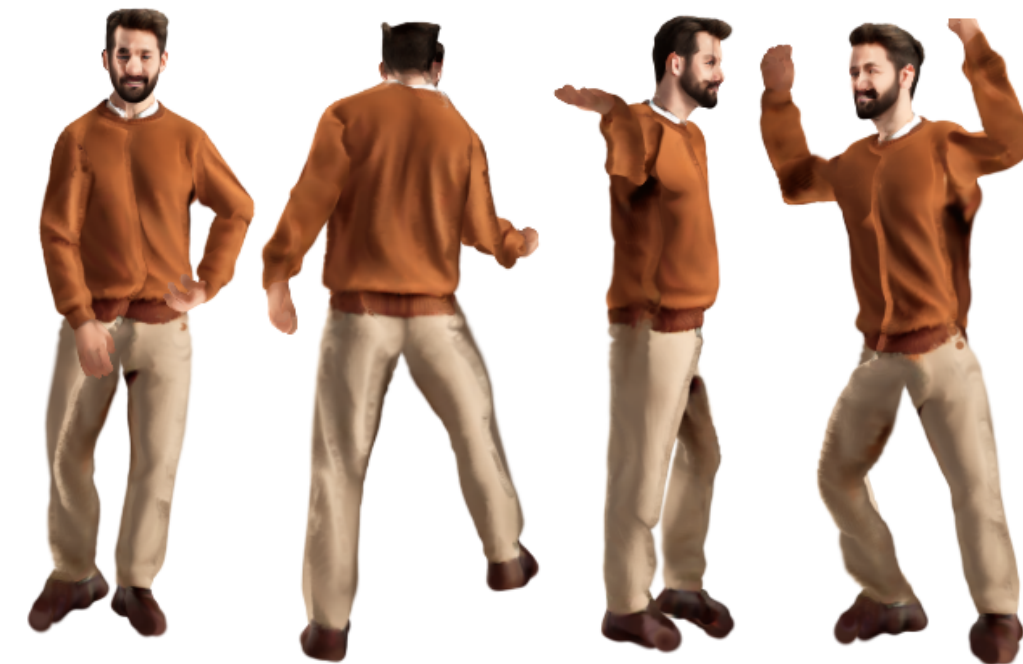

*“A man with brown seater and bright pants ”*

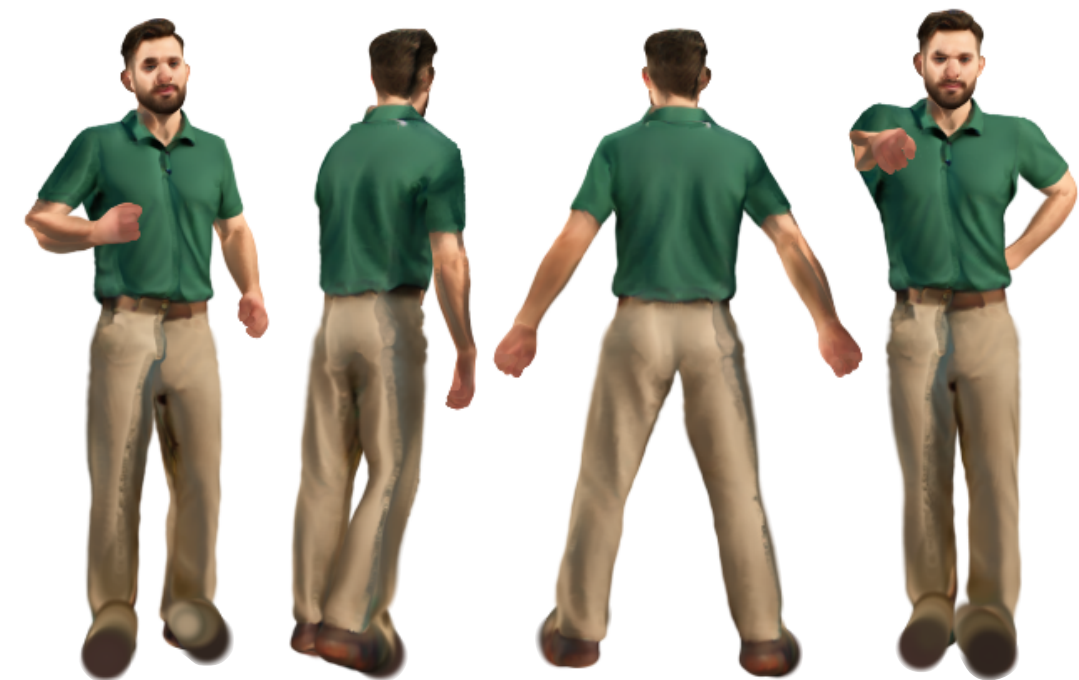

*“A man with khaki pants and green polo shirt ”*
